# Supplementary material for: Observational and Interventional Causal Learning for Regret-Minimizing Control
Source: arXiv:2212.02435 source file (2022-12-05)
Supplement: Supplementary file 1 [file appendix.tex]

% !TeX root = ../../../Main.tex

\chapter{bla}
asdf
